# Supplementary material for: Random-Access Neural Compression of Material Textures
Source: arXiv:2305.17105 source file (2023-05-26)
Supplement: Supplementary file 1 [file main_supplemental.tex]

\documentclass[acmtog, review]{acmart}
\AtBeginDocument{%
  \providecommand\BibTeX{{%
    \normalfont B\kern-0.5em{\scshape i\kern-0.25em b}\kern-0.8em\TeX}}}

\setcopyright{acmcopyright}
\copyrightyear{2023}
\acmYear{2023}
\acmDOI{XXXXXXX.XXXXXXX}

\acmConference[Conference acronym 'XX]{Make sure to enter the correct
  conference title from your rights confirmation emai}{June 03--05,
  2018}{Woodstock, NY}
\acmPrice{15.00}
\acmISBN{978-1-4503-XXXX-X/18/06}

\usepackage{xspace}
\usepackage{multirow}
\usepackage{pgfplots}
\usepackage{pgf}
\input{macros}

\begin{document}

\title{\papertitle \\ {\small Supplemental material}} %

\renewcommand{\shortauthors}{Zuppa and Panbagnato, et al.}

\begin{abstract}
This document includes supplemental material for the paper submission
``\papertitle.''
\end{abstract}

\received{20 February 2007}
\received[revised]{12 March 2009}
\received[accepted]{5 June 2009}

\maketitle

\input{supplemental.tex}

\bibliographystyle{ACM-Reference-Format}
\bibliography{bibliography}

\end{document}
